# Supplementary material for: Distributed generation of privacy preserving data with user customization
Source: arXiv:1904.09415 source file (2019-04-20)
Supplement: Supplementary file 1 [file Supplemental.tex]

\section{Latent space noise injection}
\begin{figure}[!hpbt]
    \centering
    % \includegraphics{}
    % \caption{Caption}
    % \label{fig:my_label}
\begin{tikzpicture}

  % Define nodes
  \node[obs]                               (tilde_z) {$\tilde{z}$};
  \node[latent, above=of tilde_z, xshift=-1.2cm] (z) {$ {z}$};
  \node[latent, above=of tilde_z, xshift=0.0cm]  (vareps) {$\boldsymbol{\epsilon}$};
  \node[latent, above=of tilde_z, xshift=1.2cm]  (y) {$ {y}$};
%   \node[latent, right=2cm of ]            (t) {$\tau$};

  % Connect the nodes
  \edge {z,vareps,y} {tilde_z} ; %
  %\edge {y} {vareps};

%   % Plates
%   \plate {yx} {(x)(y)} {$N$} ;
%   \plate {} {(w)(y)(yx.north west)(yx.south west)} {$M$} ;

\end{tikzpicture}
\caption{random variable graphic model. In our setting of noise injection on latent space, we yield new latent representation $\tilde{z}$ according to original latent variable $z$, random noise $\epsilon$, and sensitive label $y$.}
\label{fig:diagram:relationship}
\end{figure}
\subsection{Lower bound of information between latent embedding and sensitive label}
We hope to get a lower bound of the mutual information between original latent variable $\mathbf{z}$ and sensitive $\mathbf{y}$, denoted as $\underline{I}(z; y)$. 
First we calculate the lower bound of $I(\mathbf{z}, \mathbf{y})$, which can be expressed as follows:
\begin{align*}
    I(z; y) & = \mathbb{E}_{q(z, y)}\Big[\log q(z|y) - \log q(z) \Big] \\
    & = \mathbb{E}_{q(z, y)}\big[ \log q(z|y) - \log p(z|y) - \log q(z) + \log p(z|y) \big] \\
    & = \mathbb{E}_{q(z|y)q(y)}\big[ \log \frac{q(z|y)}{p(z|y)} \big] + \mathbb{E}_{q(z,y)} [\log p(z|y) ] - \mathbb{E}_{q(y|z)q(z)}[\log q(z)] \\
    & = \mathbb{E}_{q(y)} \Big[ D_{KL}\big(q(z|y)||p(z|y)\big) \Big]  + \mathbb{E}_{q(z,y)} [\log p(z|y) ] + H(z)\\
    & \geq \mathbb{E}_{q(z,y)} [\log p(z|y) ]  + H(z) \\
    & \triangleq \underline{I}(z; y) .
\end{align*}
The idea in the above derivation is introducing a new distribution $p(z|y)$ to approximate $q(z|y)$.  
\subsection{Upper bound of information between latent embedding and sensitive label}
We then derive an upper bound for the mutual information between the altered latent vector $\tilde{\mathbf{z}}$ and the sensitive label $\mathbf{y}$, denoted as $\overline{I}(\tilde{z}; y)$. Again we use $p(\tilde{z})$ to approximate $q(\tilde{z})$.
\begin{align*}
    I(\tilde{z}; y) & \leq I_{q(\tilde{z}, z, \varepsilon, y)}\big(\tilde{z}; (z, \varepsilon, y)\big) = \mathbb{E}_{q(\tilde{z}, z, \varepsilon, y)}\Big[\log \frac{q(\tilde{z}, z, \varepsilon, y)}{q(\tilde{z})q(z,\varepsilon, y) } \Big] \\
    & = \mathbb{E}_{q(\tilde{z}, z, \varepsilon, y)}\big[\log q(\tilde{z}|z, \varepsilon, y) - \log q(\tilde{z}) \big] \\
    & = \mathbb{E}_{q(\tilde{z}, z, \varepsilon, y)}\big[ \log q(\tilde{z}|z, \varepsilon, y) - \log p(\tilde{z}) - \log q(\tilde{z}) + \log p(\tilde{z}) \big] \\
    & = \mathbb{E}_{q(\tilde{z}| z, \varepsilon, y)q(z, \varepsilon, y)}\Big[ \log \frac{q(\tilde{z}|z, \varepsilon, y)}{p(\tilde{z})}\Big] - \mathbb{E}_{q(z, \varepsilon, y|\tilde{z})q(\tilde{z})} \big[ \log\frac{q(\tilde{z})}{p(\tilde{z})} \big] \\
    & = \mathbb{E}_{q(z, \varepsilon, y)}\Big[ D_{KL}\big( q(\tilde{z}|z, \varepsilon, y) || p(\tilde{z}) \big)\Big] - \mathbb{E}_{q(z, \varepsilon, y|\tilde{z} )} \Big[ D_{KL}\big( q(\tilde{z})||p(\tilde{z}) \big) \Big] \\
    & = \mathbb{E}_{q(z, \varepsilon, y)}\Big[ D_{KL}\big( q(\tilde{z}|z, \varepsilon, y) || p(\tilde{z}) \big)\Big] - D_{KL}\big( q(\tilde{z})||p(\tilde{z}) \big) \\
    & \leq \mathbb{E}_{q(z, \varepsilon, y)}\Big[ D_{KL}\big( q(\tilde{z}|z, \varepsilon, y) || p(\tilde{z}) \big)\Big] \\ 
    & \triangleq \overline{I}(\tilde{z}; y) . 
\end{align*}
Our goal is to verify that $\overline{I}(\tilde{z}; y) < \underline{I}(z; y) $, which ensures that the new representation $\tilde{z}$ has less information about $y$. We leverage the Monte Carlo method to calculate the expectation empirically. 

\textcolor{red}{TODO adding simulation details and results}

\break 
\textcolor{red}{TODO -Change a lot !!}
\section{Altering latent distribution via optimization}
Here we consider a general form of the data privatization game on the latent space. Specifically, denote  $q_{\phi}$ to be the distribution of the original latent variable ${z}$ and $q_{\psi}$ to be the distribution of new altered $\tilde{z}$ on space $\mathcal{Z}$. It is worth mentioning that new latent variable $\tilde{z}$ depends on $z, \epsilon, y$, that is $\tilde{z} \sim q_{\psi}(\tilde{z}|z, \epsilon, y)$. By letting the adversarial classifier $h$ and utility classifier $\nu$ play roles on latent space, we have the following canonical optimization problem: 
\begin{align}
    & \max_{q_{\psi}} \min_{h} \mathbb{E}_{\tilde{z}\sim q_{\psi}} \big[ \ell(h(\tilde{z}), y ) \big] + \beta \min_{q_{\psi}, \nu} \mathbb{E}_{\tilde{z}\sim q_{\psi}} \big[\tilde{\ell}( \nu(\tilde{z}), u) \big] \label{eq:opt:canonical:obj} \\
s.t.  & \qquad D_f(q_{\psi} || q_{\phi}) \leq \delta  \label{eq:opt:canonical:const1} 
\end{align}
where $D_f$ is the \emph{$f$-divergence} that measure the discrepancy between two distributions, $y$ and $u$ are sensitive and utility labels, and $\delta$ is divergence tolerance. The $f$ divergence between $P$ and $Q$ is $D_{f}(P||Q) = \int q(x) f\Big(\frac{p(x)}{q(x)}\Big) d\mu(x) $ (assuming $P$ and $Q$ are absolutely continuous with respect to measure $\mu$). We enumerate several examples to characterize specific constraints: 
\begin{enumerate}
    \item by taking $f(t)=t\log t$, we have KL-divergence $D_{KL}(q_{\psi} || q_{\phi}) \leq \delta $. 
    \item by taking $f(t)=-\log t $, we have reverse KL-divergence $D_{KL}(q_{\phi}|| q_{\psi} ) \leq \delta $.  
    \item by taking $f(t)= \frac{1}{2}(t-1)^2$, we have $\chi ^2$-divergence $D_{\chi^2}(q_{\psi}|| q_{\phi} ) \leq \delta$ 
    \item by taking $f(t) = \frac{t^{\alpha} - \alpha t  + \alpha - 1}{\alpha (\alpha-1)},  \alpha \in \mathbb{R} \backslash \{0,1\}  $, we have \emph{$\alpha$-divergence} $D_{\alpha}(q_{\psi}|| q_{\phi}) \leq \delta$ \cite{cichocki2010families, cichocki2009nonnegative}. As we define $f(t) = t\log t - t + 1$ when $\alpha=1$, and $f(t)=-\log t + t -1 $ when $\alpha=0$, this generalize all previous three examples (includes $\chi^2$-divergence when $\alpha=2$)
    \item note that the $\alpha$-divergence is closely related to the $\alpha$-R\'enyi divergence which has a one-to-one mapping of $f$-divergence. We use the following expression of $\alpha$-R\'enyi divergence \cite{duchi2018learning}, 
    \begin{align*}
        D_{\alpha-R}(q_{\psi}||q_{\phi}) = \frac{1}{\alpha-1}\log \int \Big( \frac{q_{\psi}}{q_{\phi}} \Big)^{\alpha} d q_{\phi} \text{ } .  
    \end{align*}
\end{enumerate}
We make connections between the current optimization formulation and some typical notions of 
\emph{differential privacy}. To disclose such links, it is worthwhile considering some typical cases in the following section \ref{sec:appx:alpha:div:diff:priv} and \ref{sec:appx:approx:diff:priv}.

\subsection{$\alpha$-divergence based privacy}\label{sec:appx:alpha:div:diff:priv}
We first consider a basic case that a vector ${z} \in \mathbb{R}^d$, let $\Pi_{\mathcal{B}_{\tau, 2}}(z)$ be the projection of the vector ${z}$ onto the $\ell_2$ ball of radius $\tau$, denoted as $\mathcal{B}_{\tau, 2}(z)$. Now, we generate the privatized latent representation $\tilde{z}$ as follows:
\begin{align}
    \tilde{z} \triangleq \frac{1}{n}\sum_{i=1}^n \Pi_{\mathcal{B}_{\tau, 2}}(z_i) + \boldsymbol{\epsilon} \label{eq:appx:noise:mech:basic:ex1}
\end{align}
where $n$ is number of samples and $\boldsymbol{\epsilon}$ is a random vector. If we denote $\zeta= \frac{1}{n}\sum_{i=1}^n \Pi_{\mathcal{B}_{\tau, 2}}(z_i)$ and $\zeta' = \frac{1}{n}\sum_{i=1}^n \Pi_{\mathcal{B}_{\tau, 2}}(z_i^{\prime})$, it is easy to discover that 
\begin{align}
    ||\zeta - \zeta' ||_2 \leq \frac{1}{n}\sum_{i=1}^n ||\Pi_{\mathcal{B}_{\tau, 2}}(z_i) - \Pi_{\mathcal{B}_{\tau, 2}}(z_i^{\prime})||_2 \leq  \frac{1}{n}\sum_{i=1}^n \min \Big\{ || z_i - z_i^{\prime} ||_2 , 2\tau \Big\}  \leq \frac{2\tau}{n} \text{card}\{ i: z_i\neq z_i^{\prime} \} \label{eq:projection:l2:bound}. 
\end{align}
When we choose $\boldsymbol{\epsilon} \sim \mathcal{N}(0, \frac{2\tau^2}{n^2 \delta} \mathbf{I} )$ where $\mathbf{I}$ is ${d\times d}$ identity matrix, and let $Q$ be the distribution of $\tilde{z}$, for samples $z_{1:n}$ and $z_{1:n}^{\prime}$ differing at most a single element (i.e. $\text{card}\{ i: z_i\neq z_i^{\prime},  \text{for } i = 1,..,n \} = 1$)
\begin{align}
    D_{\alpha}(Q(\tilde{z}|z_{1:n})||Q(\tilde{z}|z_{1:n}^{\prime})) = D_{\alpha}\Big(\mathcal{N}(\zeta, \frac{2\tau^2}{n^2 \delta} ) || \mathcal{N}(\zeta', \frac{2\tau^2}{n^2 \delta} ) \Big) = \frac{n^2\delta}{4\tau^2} ||\zeta - \zeta'||_2^2 \leq \frac{n^2\delta}{4\tau^2} \frac{4\tau^2}{n^2} = \delta,  \label{eq:alpha:gaussian:privacy}
\end{align}
where the last inequality holds because $||\zeta - \zeta'||_2 \leq \frac{2\tau}{n} $. The expression \eqref{eq:alpha:gaussian:privacy} satisfies the definition of $(\alpha, \delta)$ (R\'enyi)-differential privacy, which states that a mechanism with distribution $Q(\cdot| x)$ is ($\alpha, \delta$) R\'enyi-differential private if $D_{\alpha}\big(Q(\cdot| x)||Q(\cdot| x')\big)\leq \delta$ for all $x, x'$. \cite{mironov2017renyi}

\subsection{Approximate differential privacy}\label{sec:appx:approx:diff:priv}
We use the definition of approximate differential privacy in \cite{dwork2014algorithmic}. Namely the mechanism with conditional distribution $Q(\cdot | x)$ satisfies $(\varepsilon, \delta)$-approximate differential privacy if $Q(\cdot|x) \leq e^{\varepsilon}Q(\cdot|x') + \delta$ for all $x, x'$. We again consider the simple expression \eqref{eq:appx:noise:mech:basic:ex1} as an example. Under the Gaussian mechanism, we give a specific parameter value by using the theorem A.1 in \cite{dwork2014algorithmic}. 
% If we take  $\boldsymbol{\epsilon} \sim \mathcal{N}(0, \frac{C \log \frac{1}{\delta}}{ \varepsilon^2} \mathbf{I})$ with a particular constant $C$, then $\tilde{z}$ is ($\varepsilon, \delta$)-approximately deferentially private\cite{hall2013differential, balle2018improving}. 
 Denoting a pair of neighbouring inputs as $z \simeq z'$ and Gaussian mechanism $M(z) = f(z)+\boldsymbol{\epsilon} = \tilde{z}$ , we readdress the following theorem.
\begin{theorem}[\cite{dwork2014algorithmic}, Theorem A.1]
 For any $\varepsilon, \delta \in (0, 1)$, the Gaussian mechanism with parameter $\sigma \geq \frac{(\Delta_2f)\sqrt{2\log(\frac{1.25}{\delta})}}{\varepsilon}$ is ($\varepsilon, \delta $)-differentially private, where $(\Delta_2f) = \max_{z \simeq z'}||f(z) - f(z')||_2$ denotes the $\ell_2$-sensitivity of $f$.
\end{theorem}
The expression \eqref{eq:appx:noise:mech:basic:ex1} can be written as 
$\tilde{z} \triangleq \frac{1}{n}\sum_{i=1}^n \Pi_{\tau}(z_i) + \boldsymbol{\epsilon} = f(z) +  \boldsymbol{\epsilon}$. We have the relationship $\Delta_2 f = \frac{2\tau}{n} $ from the expression \eqref{eq:projection:l2:bound}. Therefore the Gaussian noise parameter $\sigma^2 = \frac{(\Delta_2f)^2 2 \log (1.25/\delta)}{\varepsilon^2} = \frac{8\tau^2 \log(1.25/\delta)}{n^2\varepsilon^2} $. Hence we can take $\boldsymbol{\epsilon} \sim \mathcal{N}(0, \frac{8\tau^2 \log(1.25/\delta)}{n^2\varepsilon^2} \mathbf{I})$ to ensure $\tilde{z}$ is ($\varepsilon, \delta$)-differentially private.

\textbf{Observations and Remarks}: Without considering the objectives \eqref{eq:opt:canonical:obj}, we bridge the gap between solving constrained optimization and developing differential privacy mechanisms, in the context of latent representation perturbation. In fact, by choosing the appropriate divergence with certain noise (additive) injection method and particular  parameters (such as $\varepsilon, \delta$), we discover that the $f$-divergence constraint indeed captures some cases in differential privacy. Yet the divergence based privacy in general has a weaker privacy guarantee compared with traditional $\varepsilon$- differential privacy

\subsection{Incorporating the objectives and the dual formulation}
In this part, we leverage the loss function in the objective to find an intelligent noise perturbation instead of adding noise equivalently on all coordinates as we have seen in the cases of differential privacy in \ref{sec:appx:alpha:div:diff:priv} and \ref{sec:appx:approx:diff:priv}. We change the notation to use $\theta_h$ to represent adversarial classifier $h$, and $\theta_{\nu}$ to represent utility classifier $\nu$. Because the new latent variable $\tilde{z} \sim q_{\psi}(\tilde{z}|z, \epsilon, y)$, we can rewrite the empirical loss as $\mathbb{E}_{q_{\psi}}\Big(\ell\big(\theta_h; (z, \epsilon, y) \big)\Big) = \mathbb{E}_{q_{\psi}}[\ell(h(\tilde{z}), y)]$ for sensitive labels, and similarly $\mathbb{E}_{q_{\psi}}\Big(\tilde{\ell}\big(\theta_{\nu}; (z, \epsilon, u) \big)\Big) = \mathbb{E}_{q_{\psi}}[\ell(h(\tilde{z}), u)]$ for utility labels. Thus, we express the objective \eqref{eq:opt:canonical:obj} by swap the minmax order and switch the signs as follows 
\begin{align}
    & \min_{\theta_h} \Big\{ \max_{q_{\psi}}\mathbb{E}_{q_{\psi}}\Big(\ell\big(\theta_h; (z, \epsilon, y) \big)\Big) - \beta \mathbb{E}_{q_{\psi}}\Big(\tilde{\ell}\big(\theta_{\nu}; (z, \epsilon, u) \big)\Big) \Big\} \\
    s.t. & \qquad D_f(q_{\psi}||q_{\phi}) \leq \delta \\
    & \qquad \mathbb{E} q_{\psi} = 1. \\
    & {\theta_{\nu}} = \arg\min_{\theta_{\nu}}  \mathbb{E}_{q_{\psi}}\Big(\tilde{\ell}\big(\theta_{\nu}; (z, \epsilon, u) \big)\Big)
\end{align}
It is worth noting that the constraint on $q_{\psi}$ is relevant to the inner maximization only. Thus we will derive a dual formulation based on the inner maximization for simplicity. 

\begin{theorem}\label{appx:theom:dual:obj:cvx:conjugate}
%  and a fixed mapping $g_{\psi}: (z, \epsilon, y) \mapsto \tilde{z}$ that distributed as $q_{\psi}$
 For given loss functions $\ell, \tilde{\ell}$, and certain classifiers $\theta_h, \theta_{\nu}$,  we have 
 \begin{align}
     & \max_{q_{\psi}: D_{f}(q_{\psi}||q_{\phi}) \leq \delta } \mathbb{E}_{q_{\psi}}\Big(\ell\big(\theta_h; (z, \epsilon, y) \big)\Big) - \beta \mathbb{E}_{q_{\psi}}\Big(\tilde{\ell}\big(\theta_{\nu}; (z, \epsilon, u) \big)\Big) \label{eq:app:theorm:dual:obj:original} \\
     & = \min_{\lambda > 0, \mu} \lambda \mathbb{E}_{q_{\phi}}\Big[ f^{*}\Big(\frac{\ell(\theta_h; (z, \epsilon, y)) - \beta \tilde{\ell}(\theta_{\nu}; (z, \epsilon, u)) -\mu }{\lambda}\Big) \Big] + \lambda \delta + \mu  , \label{eq:app:theorm:dual:obj:cvx:conjugate}
 \end{align}
 where $f^*$ is the Fenchel (convex) conjugate of $f$.
\end{theorem} 

\textbf{Proof:} we write the left hand-side of the equation \eqref{eq:app:theorm:dual:obj:original} in the Lagrangian form. We also re-parameterizing $dq_{\psi}/dq_{\phi} = \rho$ by leveraging the changes of the likelihood ratio that assumes $q_{\psi}$ and $q_{\phi}$ have common support.

\begin{align*}
    & \max_{q_{\psi}: D_{f}(q_{\psi}||q_{\phi}) \leq \delta }\mathbb{E}_{q_{\psi}}\Big(\ell\big(\theta_h; (z, \epsilon, y) \big)\Big) - \beta \mathbb{E}_{q_{\psi}}\Big(\tilde{\ell}\big(\theta_{\nu}; (z, \epsilon, u) \big)\Big) \\
    & = \min_{\lambda \geq 0, \mu} \max_{q_{\psi}} \int \Big[ \ell(\theta_h;(z, \epsilon, y) ) - \beta \ell(\theta_{\nu}; (z, \epsilon, u))\Big] dq_{\psi} - \lambda \Big(\int f(\frac{dq_{\psi}}{d q_{\phi}})dq_{\phi} - \delta \Big) - \mu (\int \frac{dq_{\psi}}{dq_{\phi}} dq_{\phi} - 1) \\
    & = \min_{\lambda \geq 0,\mu} \max_{q_{\psi}} \int \Big[\Big( \ell(\theta_h;(z, \epsilon, y) ) - \beta \tilde{\ell} \big(\theta_{\nu}; (z, \epsilon, u)\big) \Big) \underbrace{\frac{dq_{\psi}}{dq_{\phi}}}_{=\rho} d{q_{\phi}} - \lambda \int f(\frac{dq_{\psi}}{d q_{\phi}}) dq_{\phi} - \mu \int \frac{dq_{\psi}}{dq_{\phi}}dq_{\phi} \Big] + \lambda\delta + \mu \\
    & \explainEq{i} \min_{\lambda \geq 0,\mu} \int \lambda \max_{\rho}  \Big[\Big( \frac{\ell(\theta_h;(z, \epsilon, y) ) - \beta \tilde{\ell} \big(\theta_{\nu}; (z, \epsilon, u)\big) -  \mu }{\lambda}\Big) \rho - f(\rho) \Big] dq_{\phi} + \lambda \delta + \mu \\
    & \explainEq{ii} \min_{\lambda \geq 0,\mu } \lambda \int f^{*}\Big(\frac{\ell(\theta_h;(z, \epsilon, y) ) - \beta \tilde{\ell} \big(\theta_{\nu}; (z, \epsilon, u)\big) -  \mu  }{\lambda}\Big) dq_{\phi} + \lambda \delta + \mu \\ 
    & = \min_{\lambda \geq 0,\mu} \lambda \mathbb{E}_{q_{\phi}} \Big[ f^{*}\Big(\frac{\ell(\theta_h; (z, \epsilon, y)) - \beta \tilde{\ell}(\theta_{\nu}; (z, \epsilon, u)) -  \mu }{\lambda}\Big) \Big] + \lambda \delta + \mu,
\end{align*}
where (i) holds as we denote $dq_{\psi}/dq_{\phi} = \rho$ and rearrange the integration and maximization operations. And (ii) holds because of the Fenchel conjugate $f^*(u) = \max_{v} v^Tu - f(v)$. Therefore we convert the inner constrained maximization into an almost unconstrained minimization (with positive $\beta,\lambda$, and $\delta$). The whole objective can be simplified into 
\begin{align}
    \min_{\lambda \geq 0,\mu, \theta_h, \theta_{\nu}} \lambda \mathbb{E}_{q_{\phi}} \Big[ f^{*}\Big(\frac{\ell(\theta_h; (z, \epsilon, y)) - \beta \tilde{\ell}(\theta_{\nu}; (z, \epsilon, u)) -  \mu  }{\lambda}\Big) \Big] + \lambda \delta + \mu, \label{eq:appx:dual:obj:derived:simple}
\end{align}
given some prescribed $\beta, \lambda, \mu$, and $\delta$. 
\\

There are two major benefits to leverage the dual formulation. First, evaluating the empirical loss on the known simple distribution of $q_{\phi}$ (also known as empirical risk minimization) will be easier than evaluating loss on the unknown distribution $q_{\psi}$. Second, the convex conjugate of $f$-divergence function has convex properties that can fit nicely with (stochastic) gradient decent type method. We will leverage the following lemma to give an analytical expression of convex conjugate of $f$-divergence. 

\begin{lemma}\cite{duchi2018learning}.
If $f_\alpha(t) = \frac{t^{\alpha} - \alpha t + \alpha - 1}{\alpha(\alpha-1)}, \forall \alpha \in \mathbf{R} \backslash \{0,1 \}$, we have 
\begin{equation}
f_{\alpha}^{*}(s) = \frac{1}{\alpha} [((\alpha-1)s+1)_{+}^{\frac{\alpha}{\alpha-1}}-1] .  \label{eq:appx:duchi:robust:conj:fdiv}   
\end{equation}
\end{lemma}\label{appx:lemma:duchi:cvx:alpha:conjugate}
The proof is provided in lemma 3 of \cite{duchi2018learning}. 
\begin{corollary}
[Special case of $\alpha=0$ or $\alpha=1$] 
When $f(t) = t\log t - t + 1$, we have the Fenchel conjugate function 
\begin{align}
    f^*(s) = e^{ s} - 1. 
\end{align}
When $f(t) = -\log t + t - 1$, we have 
\begin{align}
    f^*(s) = - \log(1-s) .
\end{align} 
\end{corollary}
\textbf{Proof:} When $\alpha=1$, it boils down to $D_f(q_{\psi}||q_{\phi}) =D_{KL}(q_{\psi}||q_{\phi}) $. Because 
\begin{align*}
    D_f(q_{\psi}(z)||q_{\phi}(z))= \int q_{\phi}(z) f(\frac{q_{\psi}(z)}{q_{\phi}(z)}) dz = & \int q_{\phi} \Big( \frac{q_{\psi}}{q_{\phi}}\log \frac{q_{\psi}}{q_{\phi}} - \frac{q_{\psi}}{q_{\phi}} + 1\Big) dz \\
    = & \int q_{\psi}\log \frac{q_{\psi}}{q_{\phi}} dz - \underbrace{\int dq_{\psi}}_{=1} + \underbrace{\int dq_{\phi}}_{=1} = D_{KL}(q_{\psi}||q_{\phi}).
\end{align*}
We know $f^*(s) = \max_{t} st-f(t) = \max_{t} st-t\log t+t-1$. Taking the derivative with respect to $t$, we have $\frac{\partial(st-t\log t + t -1 )}{\partial t } = s - \log t $. As $t>0$ for the logarithmic requirement, the second order derivative $\frac{\partial(st-t\log t + t -1 )^2}{\partial ^2 t } = \frac{-1}{t} < 0$, indicating the objective is concave. We solve the maximization by letting the derivative expression $s - \log t = 0$. So $t=\exp(s)$. By substituting it into objective, we have 
\begin{align}
    f^*(s) = s\exp(s)-s\exp(s) + \exp(s) - 1 = e^s - 1 . 
\end{align}
Similarly in the case $\alpha=0$ associating with reverse KL divergence, we have $f^*(s)=\max_{t} st + \log t - t + 1 $. the first and second order derivatives are $s + \frac{1}{t} -1$ and $-1/t^2$. The objective is concave with respect to $t$. Hence we set $s + \frac{1}{t} -1=0$ to get the optimal $t$, that is $t=\frac{1}{(1-s)}$. By substituting $t$ into objective function, we have 
\begin{align}
    f^*(t)=s/(1-s) - \log(1-s) - 1/(1-s) + 1 = - \log(1-s).
\end{align}
Therefore we finish the proof. 
Combining Theorem \ref{appx:theom:dual:obj:cvx:conjugate} and Lemma \ref{appx:lemma:duchi:cvx:alpha:conjugate} together, we then automatically have the following corollary. 
\begin{corollary} Let $q_{\psi}$ be an distribution of new latent variable $\tilde{z}$ that satisfies $\tilde{z} \sim q_{\psi}(\tilde{z}|z, \epsilon, y)$. For $\alpha > 1, \delta > 0$, we have 
\begin{align*}
    & \max_{q_{\psi}: D_{f}(q_{\psi}||q_{\phi}) \leq \delta } \mathbb{E}_{q_{\psi}}\Big(\ell\big(\theta_h; (z, \epsilon, y) \big)\Big) - \beta \mathbb{E}_{q_{\psi}}\Big(\tilde{\ell}\big(\theta_{\nu}; (z, \epsilon, u) \big)\Big) \\
    = & \min_{\tilde{\mu}}\Big[c_{\alpha, \delta}\big[ \mathbb{E}_{q_{\phi}}(\ell(\theta_h; (z, \epsilon, y)) - \beta\tilde{\ell}(\theta_{\nu}; (z, \epsilon, u)) - \tilde{\mu})_{+}^{\tilde{a}}\big]^{\frac{1}{\tilde{a}}} + \tilde{\mu} \Big], 
\end{align*}
where $c_{\alpha, \delta}= \big(\alpha(\alpha-1)\delta+1\big)^{-\frac{1-\tilde{a}}{\tilde{a}}} $, and $\tilde{a} = \frac{\alpha}{\alpha-1}$.
\end{corollary}
The proof is build upon lemma 1 in \cite{duchi2018learning}. By substituting expression \eqref{eq:appx:duchi:robust:conj:fdiv} with a corresponding term in expression \eqref{eq:appx:dual:obj:derived:simple}, we immediately have the following equations
\begin{align}
    & \min_{\lambda \geq 0,\mu}\lambda\mathbb{E}_{q_{\phi}}\Big[\frac{1}{\alpha}\Big( \big[(\alpha-1)\Big(\frac{\ell(\theta_h; (z, \epsilon, y)) - \beta\tilde{\ell}(\theta_{\nu}; (z, \epsilon, u)) -\mu }{\lambda}\Big) + 1 \big]_{+}^{\frac{\alpha}{\alpha -1}} - 1 \Big) \Big] + \lambda \delta + \mu \\
   \explainEq{i}  & \min_{\lambda \geq 0,\mu} \lambda \mathbb{E}_{q_{\phi}} \Bigg[ \frac{1}{\alpha}\Big( \big[ (\frac{\alpha-1}{\lambda}) (\Delta \ell - \mu + \frac{\lambda}{\alpha-1} ) \big]_{+}^{\frac{\alpha}{\alpha-1}} - 1 \Big) \Bigg] + \lambda\delta + \mu \\
    \explainEq{ii} & \min_{\lambda \geq 0,\mu} (\alpha-1)^{\tilde{a}}  \alpha^{-1}\lambda^{1-\tilde{a}} \mathbb{E}_{q_{\phi}}\big[(\Delta \ell  - \mu + \frac{\lambda}{\alpha-1})\big]_{+}^{\tilde{a}} + (\delta - \frac{1}{\alpha})\lambda + \mu - \frac{\lambda}{\alpha-1} + \frac{\lambda}{\alpha-1} \\
    \explainEq{iii} &  \min_{\lambda \geq 0,\mu} (\alpha-1)^{\tilde{a}}  \alpha^{-1}\lambda^{1-\tilde{a}} \mathbb{E}_{q_{\phi}}(\Delta \ell - \tilde{\mu})_{+}^{\tilde{a}} + (\delta + \frac{1}{\alpha(\alpha-1)})\lambda + \tilde{\mu}, \label{eq:appx:obj:reparam:dual:min:tilde_a}
\end{align}
where (i) holds because we denote $\ell(\theta_h; (z, \epsilon, y)) - \beta\tilde{\ell}(\theta_{\nu}; (z, \epsilon, u))=\Delta\ell$, (ii) is valid because we let $\tilde{a} = \frac{\alpha}{\alpha-1}$, and (iii) holds because we denote $\tilde{\mu} = \mu - \frac{\lambda}{\alpha-1}$. It's not difficult to discover that the function \eqref{eq:appx:obj:reparam:dual:min:tilde_a} is convex with respect to $\lambda$. Taking the derivative of  \eqref{eq:appx:obj:reparam:dual:min:tilde_a} with respect to $\lambda$ and set it to 0, we have $\lambda^* = (\alpha(\alpha-1)\delta + 1)^{-\frac{1}{\tilde{a}}}(\alpha-1)\big[\mathbb{E}_{q_{\phi}}(\Delta\ell - \tilde{\mu})^{\tilde{a}} \big]^{\frac{1}{\tilde{a}}}$. By replacing the $\lambda$ with the optimal value in \eqref{eq:appx:obj:reparam:dual:min:tilde_a}, we can simplify the objective function as 
\begin{align}
    & \min_{\tilde{\mu}} \big(\alpha(\alpha-1)\delta+1\big)^{-\frac{1-\tilde{a}}{\tilde{a}}} \big[ \mathbb{E}_{q_{\phi}}(\Delta \ell - \tilde{\mu})_{+}^{\tilde{a}}\big]^{\frac{1}{\tilde{a}}} + \tilde{\mu} \\ 
    = & \min_{\tilde{\mu}}\Big[c_{\alpha, \delta}\big[ \mathbb{E}_{q_{\phi}}(\ell(\theta_h; (z, \epsilon, y)) - \beta\tilde{\ell}(\theta_{\nu}; (z, \epsilon, u)) - \tilde{\mu})_{+}^{\tilde{a}}\big]^{\frac{1}{\tilde{a}}} + \tilde{\mu} \Big]
\end{align}
where $c_{\alpha, \delta}= \big(\alpha(\alpha-1)\delta+1\big)^{-\frac{1-\tilde{a}}{\tilde{a}}} $. Thus we finish the proof of the corollary.

% \textcolor{red}{TODO...
% With such a simplified optimization, we succinctly express the loss as 
% }

% \begin{align}
%     \min_{\theta_{h}, \theta_{\nu}, \tilde{\mu}}
% \end{align}

Such a unified optimization allows us to explore different divergence constraints such as $D_{KL}$ or $\chi^2$ with particular choices of $\alpha$.

% \min_{\lambda \geq 0, \theta_h, \theta_{\nu}} \mathbb{E}_{q_{\phi}} \Big[ f^{*}\Big(\frac{\ell(\theta_h; (z, \epsilon, y)) - \beta \tilde{\ell}(\theta_{\nu}; (z, \epsilon, u)) }{\lambda}\Big) \Big]     
% \end{equation}

\subsection{KL- and $\chi^2$-divergence for two multivariate Gaussian}
In this section, we consider two special cases of divergences that are $D_{KL}$ and $\chi^2$ of two distribution $P$ and $Q$. Specifically, we assume both $P$ and $Q$ are multivariate Gaussian distribution with mean $\mu_1, \mu_2 $ and covariance $\Sigma_1, \Sigma_2$ to simplify our models. Specifically, for $d$-dimensional Gaussian distribution $P$ has the density  
\begin{align*}
    P(x) = \frac{1}{(2\pi)^{\frac{d}{2}} |\Sigma_1|^{\frac{1}{2}} } \exp\Big( -\frac{1}{2}(x-\mu_1)^T\Sigma_1^{-1}(x-\mu_1) \Big)
\end{align*}

We simplify our parameter regularization by giving a specific analytic expression as follows. 

\begin{align*}
   & D_{KL}(P||Q)  = \mathbb{E}_P[\log\frac{P}{Q}]\\
    & = \frac{1}{2}\mathbb{E}_P\Big[ - \log |\Sigma_1| - (x-\mu_1)^T\Sigma_1^{-1}(x-\mu_1) + \log |\Sigma_2| + (x-\mu_2)^T\Sigma_2^{-1}(x-\mu_2)\Big] \\
    & = \frac{1}{2} \Big(\log |\Sigma_2|-\log|\Sigma_1| - d + \Tr(\Sigma_2^{-1}\Sigma_1) + (\mu_1-\mu_2)^T\Sigma_2^{-1}(\mu_1 -\mu_2)\Big). 
\end{align*}

\begin{align*}
    & D_{\chi^2}(P||Q)  = E_{Q}[\frac{1}{2}(\frac{P}{Q}-1)^2] \\
    & =  \frac{1}{2}\Bigg[ \frac{|\Sigma_2|}{|\Sigma_1|} \exp\big(-\Tr(\Sigma_1^{-1}\Sigma_2) + d - \mu_1^T\Sigma_1^{-1}\mu_1 - \mu_2^T\Sigma_2^{-1}\mu_2 + 2\mu_1^T\Sigma_1^{-1}\mu_2 \big) \\ 
    & - \frac{|\Sigma_2|^{\frac{1}{2}}}{|\Sigma_1|^{\frac{1}{2}}} \exp\big(-\frac{1}{2}\Tr(\Sigma_1^{-1}\Sigma_2) + \frac{d}{2}  -\frac{1}{2}\mu_1^T\Sigma_1^{-1}\mu_1 - \frac{1}{2}\mu_2^T\Sigma_2^{-1}\mu_2 + \mu_1^T\Sigma_1^{-1}\mu_2 \big) + 1\Bigg] \\
    & = \frac{1}{2}\Big[ \exp\big( \log\frac{|\Sigma_2|}{|\Sigma_1|}  -\Tr(\Sigma_1^{-1}\Sigma_2) + d - \mu_1^T\Sigma_1^{-1}\mu_1 - \mu_2^T\Sigma_2^{-1}\mu_2 + 2\mu_1^T\Sigma_1^{-1}\mu_2  \big) \\ 
    & - 2\exp\Big(\frac{1}{2}\big(\log\frac{|\Sigma_2|}{|\Sigma_1|} - \Tr(\Sigma_1^{-1}\Sigma_2) + d - \mu_1^T\Sigma_1^{-1}\mu_1 - \mu_2^T\Sigma_2^{-1}\mu_2 + 2\mu_1^T\Sigma_1^{-1}\mu_2 \big) \Big) + 1 \Big] \\
    & \explainEq{i} \frac{1}{2}\bigg(\exp \big[\underbrace{d + (2\mu_2 - \mu_1)^T\Sigma_1^{-1}\mu_1 - \mu_2^T\Sigma_2^{-1}\mu_2}_{s}\big] - 2 \exp\big[\underbrace{\frac{d + (2\mu_2 - \mu_1)^T\Sigma_1^{-1}\mu_1  - \mu_2^T\Sigma_2^{-1}\mu_2}{2}}_{s/2}\big] + 1 \bigg) \\
    & \explainEq{ii} \frac{1}{2}\big(\exp(s/2)-1\big)^2. 
\end{align*}
(i) holds as $\log\frac{|\Sigma_2|}{|\Sigma_1|} = \log |\Sigma_1^{-1}\Sigma_2|= \Tr (\Sigma_1^{-1}\Sigma_2)$. (ii) as we denote $s = d + (2\mu_2 - \mu_1)^T\Sigma_1^{-1}\mu_1 - \mu_2^T\Sigma_2^{-1}\mu_2$. In the VAE setting, we treat the covariance matrix as the diagonal form $\Sigma = \diag\begin{bmatrix} \sigma_1, \dots, \sigma_d \end{bmatrix}$. The inverse and determinant of the covariance will be simplified as
$\Sigma^{-1} = \diag[1/\sigma_1, \dots, 1/\sigma_d]$ and  $|\Sigma| = \prod_{i=1}^d \sigma_i$.

% \subsection{} 

% \break 

% \input{Connection_to_adversarial.tex}
